# Supplementary material for: A GRU-based Mixture Density Network for Data-Driven Dynamic Stochastic Programming
Source: arXiv:2006.16845 source file (2020-06-26)
Supplement: Supplementary file 1 [file appendix.tex]

\appendix
\section{Proof of Proposition \ref{p1}}

\begin{proof}
The SUBP can be treated as min-cost flow problem on the directed graph $\mathscr{N}$ 
\end{proof}
